# Supplementary material for: Joint Wasserstein Distribution Matching
Source: arXiv:2003.00389 source file (2020-03-01)
Supplement: Supplementary file 1 [file appendix.tex]

\section{Appendix}

%\paragraph{Wasserstein Distance of Joint Distributions.} 
To address the joint distribution matching problem, we assume a shared latent space $ \gZ $ in two domains~\cite{liu2017unsupervised}.
%one can learn a shared latent space $ \gZ $ in two domains~\cite{liu2017unsupervised}.
%In this sense, 
It means that any pair of images in different domains can be mapped to the same latent representation. 
Inversely, there exist generative models $ P_{G_1}(X'|Z) $ and $ P_{G_2}(Y'|Z) $ that map a shared latent code $ Z $ to $ X' {=} G_1(Z) $ and $ Y' {=} G_2(Z) $, respectively.
Then $ P_{\gA} (X, Y') $ and $ P_{\gB} (X', Y) $ are two joint distributions between real and generated images.
%we define Wasserstein distance $ \gW_c(P_{\gA},  P_{\gB}) $ as %between joint distributions $ P_{\gA} $ and $ P_{\gB} $, \textit{i.e.},
%\begin{align} \label{pro:joint_ot}
%\gW_c(P_{\gA},  P_{\gB}) \mathop{=} \min_{P {\in} \gP(P_{\gA}, P_{\gB})}
%\E_{P} [c(X, Y'; X', Y)],
%\end{align}
%where $ \gP(P_{\gA}, P_{\gB}) $ is the set of couplings composed of joint  distributions with the probability distributions $ (P_{\gA},  P_{\gB}) $. %, and $ c $ is a  cost function. 
%In practice, we set the cost function $ c(X, Y'; X', Y) = c_1(X, X') + c_2(Y', Y) $ \cite{damodaran2018deepjdot}, where $ c_1 $ and $ c_2 $ can be any metric.
%{However, directly optimizing Problem (\ref{pro:joint_ot})  would incur intractable computation cost and statistical difficulties~\cite{genevay2018learning}.  To address this, we first reduce the intractable Problem (\ref{pro:joint_ot}) into a simpler optimization problem using Theorem \ref{thm:opt} below.}  
\kui{Let $ Q(Z_1|X) $ and $ Q(Z_2|Y) $ be two probabilistic encoders,} where $ X {\sim} P_{X}  $ and $ Y {\sim} P_{Y} $,
and $ Q_{Z_1} $ and $ Q_{Z_2} $ be two marginal distributions: \cao{$Q_{Z_1} {=} \E_{P_X}[Q(Z_1|X)]$ and $Q_{Z_2} {=} \E_{P_Y}[Q(Z_2|Y)]$}.  %of $ Z_1 {\sim} Q(Z_1|X) $ and $ Z_2 {\sim} Q(Z_2|Y) $, respectively
%Then, we can achieve an equivalent problem to Problem (\ref{pro:joint_ot}) as follows.
Then, we solve an equivalent problem using the following theorem. %to Problem (\ref{problem:Wasserstein_jd})

\begin{thm} \emph{\textbf{(Problem equivalence)}}  \label{thm:opt}
	Given two deterministic models $ P_{G_1} (X'|Z) $ and $ P_{G_2} (Y'|Z) $ as Dirac measures, \textit{i.e.},
	$ P_{G_1}({X'}|Z{=}\rvz){=}\delta_{G_1(\rvz)} $ and $ P_{G_2}(Y'|Z{=}\rvz){=}\delta_{G_2(\rvz)} $ for all $ \rvz {\in} \gZ $, we can rewrite Problem (\ref{problem:Wasserstein_jd}) as follows:
	\begin{align} \label{obj:w}
	\gW_c(P_{\gA}, P_{\gB})
	{=}& \inf_{Q  {\in} \gQ_1} \E_{P_{X}} \E_{Q{(Z_1|X)}}  [c_1(X, G_1(Z_1))] \\
	&\tiny{+}\inf_{Q {\in} \gQ_2} \E_{P_{Y}} \E_{Q{(Z_2|Y)}} [c_2(G_2(Z_2), Y)]. \nonumber
	\end{align}
	where we define $ \gQ_1 {=} \{Q(Z_1|X) |\; Q {\in} \tilde{\gQ}, P_Y {=} Q_{Y} \} $ and $ \gQ_2 {=} \{Q(Z_2|Y) |\; Q {\in} \tilde{\gQ}, P_X {=} Q_{X} \} $ as the sets of all probabilistic encoders, respectively,  \cao{where $Q$ satisfies the set $\tilde{\gQ} {=} \{ Q| P_{Z_1} {=} Q_{Z_1}, P_{Z_2} {=} Q_{Z_2} \} $}. In practice, we set the cost function $ c(X, Y'; X', Y) {=} c_1(X, X') {+} c_2(Y', Y) $ \cite{damodaran2018deepjdot}, where $ c_1 $ and $ c_2 $ can be any metric.
\end{thm}
\begin{proof}
See supplementary materials for the proof.
\end{proof}
