# Supplementary material for: Joint Wasserstein Distribution Matching
Source: arXiv:2003.00389 source file (2020-03-01)
Supplement: Supplementary file 2 [file supp_backups.tex]

\onecolumn
\vskip 0.3in
\clearpage
\textbf{\Large{~~~~~Supplementary Materials for ``Joint Wasserstein Distribution Matching''}}
\vspace{20pt}
%\begin{Large}
% 	~~~~~~~~~~Supplementary Materials for ``Joint Wasserstein Distribution Matching''
%% 	~~~~~~~~~~~~{\large{Supplementary Materials}}: ``J{\large{OINT}} W{\large{ASSERSTEIN}} D{\large{ISTRIBUTION}}-E{\large{ATCHING}}''
%\end{Large}
%\title{Joint Wasserstein Distribution Matching}
%\begin{appendix}

\setcounter{section}{0}

\section{Theoretical Analysis}\label{sec:theory}  %Wasserstein Distance of Joint Distributions
%{To learn a joint distribution, one can learn a shared latent space for two different domains~\citep{liu2017unsupervised}.}
%%Based on the shared-latent space assumption~\citep{liu2017unsupervised}, 
%In this sense, any pair of images in different domains can be mapped to the same latent representation. % in a shared-latent space.
%We define latent variable models $ P_{G_1} $ and $ P_{G_2} $ by a two-step procedure: first a code $ Z {\in} \gZ $ is sampled from some prior distribution $ P_{Z} $ and then $ Z $ can be mapped to $ X $ and $ Y $, respectively. 
%Then, we have the following densities:% of the form:
%\begin{align}\label{eq:G1G2}
%	p_{G_1}(\rvx) {:=} \int_{\gZ} p_{G_1}(\rvx|\rvz) p_{\rvz}(\rvz) d\rvz, \forall\; \rvx {\in} \gX, \quad\;
%	p_{G_2}(\rvy) {:=} \int_{\gZ} p_{G_2}(\rvy|\rvz) p_{\rvz}(\rvz) d\rvz, \forall\; \rvy {\in} \gY,
%\end{align}
%where all involved densities are properly defined.
%In this paper, we focus on non-random decoders $ G_1{:\;} \gZ {\to} \gX $ and $ G_2{:\;} \gZ {\to} \gY $, \textit{i.e.}, generative models $ P_{G_1}(X'|Z) $ and $ P_{G_2}(Y'|Z) $ deterministically mapping $ Z $ to $ X' {=} G_1(Z) $ and $ Y' {=} G_2(Z) $, respectively.
%Based on these two models, we then construct joint distributions in two domains and define the following Wasserstein distance.
%
To address the joint distribution matching problem, one can learn a shared latent space $ \gZ $ in two domains~\cite{liu2017unsupervised}.
In this sense, any pair of images in different domains can be mapped to the same latent representation. 
Inversely, there exist generative models $ P_{G_1}(X'|Z) $ and $ P_{G_2}(Y'|Z) $ that map a shared latent code $ Z $ to $ X' {=} G_1(Z) $ and $ Y' {=} G_2(Z) $, respectively.
%\textbf{Wasserstein distance between joint distributions.}
Then $ P_{\gA} (X, Y') $ and $ P_{\gB} (X', Y) $ are two joint distributions between real and generated images, 
%, where $ X' $ and $ Y' $ are sampled from the models $ {G_1} $ and $ {G_2} $, respectively, and $ X $ and $ Y $ are true images from different domains.
%For the unsupervised joint distribution matching problem,
%Based on the optimal transport theory~\cite{villani2008optimal}, 
we define Wasserstein distance $ \gW_c(P_{\gA},  P_{\gB}) $ as %between joint distributions $ P_{\gA} $ and $ P_{\gB} $, \textit{i.e.},
%Our goal is to find a optimal coupling to make these two joint distributions to close to each other.
\begin{align} \label{pro:joint_ot}
\gW_c(P_{\gA},  P_{\gB}) \mathop{=} \min_{P {\in} \gP(P_{\gA}, P_{\gB})}
\E_{P} [c(X, Y'; X', Y)],
\end{align}
where $ \gP(P_{\gA}, P_{\gB}) $ is the set of couplings composed of joint  distributions with the probability distributions $ (P_{\gA},  P_{\gB}) $. %, and $ c $ is a  cost function. 
In practice, we set the cost function $ c(X, Y'; X', Y) = c_1(X, X') + c_2(Y', Y) $ \cite{damodaran2018deepjdot}, where $ c_1 $ and $ c_2 $ can be any metric.
% between two joint probability distributions $ P_{\gA} $ and $ P_{\gB} $.
%When $ (\gX {\times} \gY)^2 $ is equipped with a metric $ d $, a typical choice is to set $ c (\rvx, \rvy'; \rvx', \rvy) {=} d(\rvx, \rvy'; \rvx', \rvy)^p $, where $ p > 0 $. For $ p \ge 1 $, $ \gW^p(P_{\gA},  P_{\gB}) $ is the $ p $-Wasserstein distance between the probability distributions $ (P_{\gA},  P_{\gB}) $.
%there are an important challenges on Wasserstein distance and the cost function.
\kui{However, directly optimizing Problem (\ref{pro:joint_ot})  would incur intractable computation cost and statistical difficulties~\cite{genevay2018learning}.  To address this, we first reduce the intractable Problem (\ref{pro:joint_ot}) into a simpler optimization problem using the following Theorem \ref{thm:opt}.}  \\
%To address this, we need to propose a new optimization method for our problem setting.
%in the unsupervised image-to-image translation task.
%Second, how to choose a appropriate cost function is very challenging.
%In this paper, we set $ c(X, Y'; X', Y) = c_1(X, X') + c_2(Y', Y) $~\citep{damodaran2018deepjdot}, where $ c_1 $ and $ c_2 $ can be any metric to measure the distance in $ \gX {\times} \gX $ and $ \gY {\times} \gY $, respectively. 
%This cost function 
%Here, we set $ \lambda{=}1 $ for convenience.
%, and $ \lambda $ is a positive parameter which balances $ c_1 $ and $ c_2 $ in the their corresponding feature spaces.
%\cao{Then, we derive the following theorem so that the intractable Problem (\ref{pro:joint_ot}) can be reduced to a simple optimization problem.}
%\kui{Give more clear definitions about $Q$ here!!!} 
\emph{
\noindent\textbf{\emph{Theorem \ref{thm:equ_problem}}} (\textbf{Problem equivalence})
	Assume that two domains share the same latent space, then Wasserstein distribution between joint distributions can be defined as
	\begin{equation}
	\begin{aligned}  \label{prob:equ_problem}
	\gW_c(\gP_{\gA}, \gP_{\gB}) &= \gR_x(F) + \gR_y(F), \\
	\st \quad P_X &= Q_X, P_Y = Q_Y, P_Z = Q_Z,
	\end{aligned}
	\end{equation}
	where $ \gR_x (F)$ and $\gR_y(F) $ are reconstruction losses \wrt Auto-Encoders $ G_1{\circ} E_1 $ and $ G_2 {\circ} E_2 $. For convenience, we let $ F{=}\{E_1, E_2, G_1, G_2\} $. Here, $ P_X, P_Y $ and $ P_Z $ are real distributions, and $ Q_X, Q_Y $ and $ Q_Z $ are generated distributions.
}

\begin{proof}
From Theorem \ref{thm:opt}, we define the reconstruction losses as:
\begin{align*}
	\gR_x(F) = \E_{P_{X}} \E_{Q{(Z_1|X)}}  [c_1(X, G_1(Z_1))]\quad \text{and} \quad \gR_y(F) = \E_{P_{Y}} \E_{Q{(Z_2|Y)}} [c_2(G_2(Z_2), Y)],
\end{align*}
where $ c_1(X, G_1(Z_1))=\| X- G_1(Z_1) \|_1 $ and $ c_2(G_2(Z_2), Y)=\| G_2(Z_2)- Y \|_1 $ in this paper. 
For the constraints in this problem, we enforce the constraints in Theorem \ref{thm:opt}, $ P_X {=} Q_X, P_Y {=} Q_Y $ and $ P_{Z_1}{=}Q_{Z_1}, P_{Z_2}{=}Q_{Z_2} $. 
Note that $ P_{Z_1} {=} P_{Z_2} $, and they are prior distributions. 
We let $ P_Z{:=} \{P_{Z_1}, P_{Z_2}\} $ and $ Q_Z{:=} \{Q_{Z_1}, Q_{Z_2} \} $, then we have $ P_Z = Q_Z $.

\end{proof}
%\vspace{15pt}


\kui{Let $ Q(Z_1|X) $ and $ Q(Z_2|Y) $ be two probabilistic encoders,} where $ X {\sim} P_{X}  $ and $ Y {\sim} P_{Y} $,
and $ Q_{Z_1} $ and $ Q_{Z_2} $ be two marginal distributions: \cao{$Q_{Z_1} {=} \E_{P_X}[Q(Z_1|X)]$ and $Q_{Z_2} {=} \E_{P_Y}[Q(Z_2|Y)]$}.  %of $ Z_1 {\sim} Q(Z_1|X) $ and $ Z_2 {\sim} Q(Z_2|Y) $, respectively
% We define the sets of all probabilistic encoders as $ \gQ_1 {=} \{Q(Z_1|X) |\; Q {\in} \tilde{\gQ}, P_Y {=} Q_{Y} \} $, $ \gQ_2 {=} \{Q(Z_2|Y) |\; Q {\in} \tilde{\gQ}, P_X {=} Q_{X} \} $ \cao{where $Q$ satisfies the set $\tilde{\gQ} {=} \{ Q| P_{Z_1} {=} Q_{Z_1}, P_{Z_2} {=} Q_{Z_2} \} $}. %
Then, we can achieve an equivalent problem to Problem (\ref{pro:joint_ot}) as follows.

\begin{thm}\label{thm:opt}
	Given two deterministic models $ P_{G_1} (X'|Z) $ and $ P_{G_2} (Y'|Z) $ as Dirac measures, \textit{i.e.},
	$ P_{G_1}({X'}|Z{=}\rvz){=}\delta_{G_1(\rvz)} $ and $ P_{G_2}(Y'|Z{=}\rvz){=}\delta_{G_2(\rvz)} $ for all $ \rvz {\in} \gZ $, we can rewrite Problem (\ref{pro:joint_ot}) as follows:
	%\begin{equation}
	%\begin{aligned}\label{obj:w}
	\begin{align} \label{obj:w}
	\gW_c(P_{\gA}, P_{\gB})
	{=}& \inf_{Q  {\in} \gQ_1} \E_{P_{X}} \E_{Q{(Z_1|X)}}  [c_1(X, G_1(Z_1))] \\
	&\tiny{+}\inf_{Q {\in} \gQ_2} \E_{P_{Y}} \E_{Q{(Z_2|Y)}} [c_2(G_2(Z_2), Y)], \nonumber
	\end{align}
	where we define $ \gQ_1 {=} \{Q(Z_1|X) |\; Q {\in} \tilde{\gQ}, P_Y {=} Q_{Y} \} $ and $ \gQ_2 {=} \{Q(Z_2|Y) |\; Q {\in} \tilde{\gQ}, P_X {=} Q_{X} \} $ as the sets of all probabilistic encoders, respectively,  \cao{where $Q$ satisfies the set $\tilde{\gQ} {=} \{ Q| P_{Z_1} {=} Q_{Z_1}, P_{Z_2} {=} Q_{Z_2} \} $}.
	%\end{aligned}
	%\end{equation}
	%\footnote{See supplementary materials for the proof.}
\end{thm}


% \begin{remark}
%     Theorem \ref{thm:opt} indicates that Problem \ref{obj:w} is equivalent to Problem \ref{pro:joint_ot}. 
%     %$  G_2{\circ}E_1  $ and $  G_1 {\circ}E_2 $ to generate samples $ Y' $ and $ X' $ such that the generated distribution is close to real distribution.
%     Moreover, latent distributions learned by two probabilistic encoders (\ie ) should be close to each other.
% \end{remark}

%As previously mentioned, finding an optimal couplings between $ P_{\gA} $ and $ P_{\gB} $ is very challenging. Fortunately, according to Theorem \ref{thm:opt}, we can instead optimize problem (\ref{obj:w}) for joint distribution matching. 
%The objective function and detailed optimizations are given below.
%Theorem \ref{thm:opt} allows us to construct an optimization problem by optimizing $ Q(Z_1|X) $ and $ Q(Z_2|Y) $ instead of finding an optimal couplings between joint distributions $ P_{\gA} $ and $ P_{\gB} $.

\begin{proof}
	We denote by $ \gP(X {\sim} P_X, {X'} {\sim} P_{G_1}) $ and $ \gP(Y {\sim} P_Y, {Y'} {\sim} P_{G_2}) $ the set of all joint distributions of $ (X, {X'}) $ and $ (Y, {Y'}) $ with marginals $ P_X, P_{G_1} $ and $ P_Y, P_{G_2} $, respectively,
	and denote by $ \gP(P_{\gA}, P_{\gB}) $ the set of all joint distribution of $ P_{\gA} $ and $ P_{\gB} $. Recall the definition of Wasserstein distance $ \gW_c(P_{\gA}, P_{\gB}) $, we have
	\begin{align}
	\gW_c(P_{\gA}, P_{\gB}) 
	=& \inf_{\pi \in \gP(P_{\gA}, P_{\gB})} \E_{(X, Y'; X', Y) \sim \pi} [ c(X, Y'; X', Y)] \label{eqn:AE1}\\
	=& \inf_{\pi \in \gP(P_{\gA}, P_{\gB})} \E_{(X, Y'; X', Y) \sim \pi} [ c_1(X, X') ] 
	+ \inf_{\pi \in \gP(P_{\gA}, P_{\gB})} \E_{(X, Y'; X', Y) \sim \pi} [ c_2(Y', Y) ] \nonumber \\
	=& \inf_{P \in \gP_{X, X'}} \E_{(X, X') \sim P} [c_1(X, X')] 
	+ \inf_{P \in \gP_{Y, Y'}} \E_{(Y', Y) \sim P} [ c_2(Y', Y)] \label{eqn:AE2}\\
	=& \inf_{P \in \gP({P_{X}, P_{G_1}})} \E_{(X, X') \sim P} [c_1(X, X')] 
	+ \inf_{P \in \gP({P_{Y}, P_{G_2}})} \E_{(Y', Y) \sim P} [ c_2(Y', Y)] \label{eqn:AE3}\\
	=& \;\gW_{c_1}(P_{X}, P_{G_1}) +  \gW_{c_2}(P_{G_2}, P_{Y}). \nonumber
	\end{align}
	Line (\ref{eqn:AE1}) holds by the definition of $ \gW_c(P_{\gA}, P_{\gB})  $.
%	The second line holds by the choose of the ground cost, \textit{i.e.}, $ c(X, Y'; X', Y ) {=}  c_1(X, X') +  c_2(Y', Y) $. 
	Line (\ref{eqn:AE2}) uses the fact that the variable pair $ (X, X') $ is independent of the variable pair $ (Y, Y') $, and $ \gP_{X, X'} $ and $ \gP_{Y, Y'} $ are the marginals on $ (X, X') $ and $ Y, Y' $ induced by joint distributions in $ \gP_{X, Y', X', Y} $. 
	In Line (\ref{eqn:AE3}), if $ P_{G_1}(X'|Z) $ and $ P_{G_2}(Y'|Z) $ are Dirac measures (\textit{i.e.}, $ X' {=} G_1(Z) $ and $ Y' {=} G_2(Z) $), we have 
	\[\gP_{X, X'} {=} \gP(P_X, P_{G_1}), \qquad \gP_{Y, Y'} {=} \gP(P_Y, P_{G_2}). \]
	We consider certain sets of joint probability distributions $ \gP_{X, X', Z_1} $ and $ \gP_{Y, Y', Z_2} $ of three random variables $ (X, X', Z_1) \in \gX {\times} \gX {\times} \gZ $ and $ (Y', Y, Z_2) \in \gY {\times} \gY {\times} \gZ $, respectively. 
	%	We denote by $ P_{G_1, Z}(X', Z) $ and $ P_{G_2, Z}(Y', Z) $ joint distributions of variable pairs $ (X', Z) $ and $ (Y', Z) $, respectively, where $ Z $ is first sampled from $ P_Z $ and then $ X' $ from $ P_{G_1}(X'|Z) $ and $ Y' $ from $ P_{G_2}(Y'|Z) $, respectively.
	%	Note that $ P_{G_1} $ and $ P_{G_2} $ defined in (\ref{eq:G1G2}) are the marginal distributions of $ X' $ and $ Y' $ when $ (X', Z) {\sim} P_{G_1, Z} $ and $ (Y', Z) {\sim} P_{G_2, Z} $.
	We denote by $ \gP(X {\sim} P_X, Z_1 {\sim} P_{Z_1}) $ and $ \gP(Y {\sim} P_Y, Z_2 {\sim} P_{Z_2}) $ the set of all joint distributions of $ (X, Z_1) $ and $ (Y, Z_2) $ with marginals $ P_X, P_{Z_1} $ and $ P_Y, P_{Z_2} $, respectively.
	The set of all joint distributions $ \gP_{X, X', Z_1} $ such that $ X {\sim} P_X, (X', Z_1) {\sim} P_{G_1, Z_1} $ and $ (X' {\Perp} X) | Z_1 $, and likewise for $ \gP_{Y, Y', Z_2} $.
	We denote by $ \gP_{X, X'} $ and $ \gP_{X, Z_1} $ the sets of marginals on $ (X, X') $ and $ (X, Z_1) $ induced by distributions in $ \gP_{X, X', Z_1} $, respectively, and likewise for $ \gP_{Y, Y'} $ and $ \gP_{Y, Z_2} $.
	%	Since the latent variable $ Z $ is related to $ P_{G_1} $ and $ P_{G_2} $, we 
	For the further analyses, we have
%	\begin{small}
	\begin{align}
	&\gW_{c_1}(P_{X}, P_{G_1}) +  \gW_{c_2}(P_{Y}, P_{G_2}) \nonumber\\
	{=}& \inf_{P \in \gP_{X, X', Z_1}} \E_{(X, X', Z_1) \sim P} [ c_1(X, X') ] \label{eqn:ae1}
	 {+} \inf_{P \in \gP_{Y', Y, Z_2}} \E_{(Y', Y, Z_2) \sim P} [  c_2(Y', Y) ]  \\
	{=}& \inf_{P \in \gP_{X, X', Z_1}} \E_{P_{Z_1}} \E_{X \sim P(X|Z_1)} \E_{X' \sim P(X'|Z_1)} [ c_1(X, X') ] \label{eqn:ae2} \\
	 &{+} \inf_{P \in \gP_{Y', Y, Z_2}} \E_{P_{Z_2}} \E_{Y \sim P(Y|Z_2)} \E_{Y' \sim P(Y'|Z_2)} [ c_2(Y', Y) ] \nonumber \\
	{=}& \inf_{P \in \gP_{X, X', Z_1}} \E_{P_{Z_1}} \E_{X \sim P(X|Z_1)} [ c_1(X, G_1(Z_1)) ] 
	 {+} \inf_{P \in \gP_{Y', Y, Z_2}} \E_{P_{Z_2}} \E_{Y \sim P(Y|Z_2)} [ c_2(G_2(Z_2), Y) ] \nonumber \\
	{=}& \inf_{P \in \gP_{X, Z_1}} \E_{(X, Z_1) \sim P} [ c_1(X, G_1(Z_1)) ]  
	 {+} \inf_{P \in \gP_{Y, Z_2}} \E_{(Y, Z_2) \sim P} [ c_2(G_2(Z_2), Y) ] \label{eqn:ae4} \\
	{=}& \inf_{P \in \gP(X, Z_1)} \E_{(X, Z_1) {\sim} P} [ c_1(X, G_1(Z_1)) ] 
	 {+} \inf_{P \in \gP(Y, Z_2)} \E_{(Y, Z_2) {\sim} P} [ c_2(G_2(Z_2), Y) ] \label{eqn:ae5} \\
	{=}& \inf_{Q \in \gQ_1} \E_{P_{X}} \E_{Q{(Z_1|X)}} [c_1(X, G_1(Z_1))] 
	 {+} \inf_{Q \in \gQ_2} \E_{P_{Y}} \E_{Q{(Z_2|Y)}} [c_2(G_2(Z_2), Y)], \label{eqn:ae6} 
	\end{align}
%	\end{small}
	where $ \gQ_1 {=} \{Q(Z_1|X) | Q_{Z_1} {=} P_Z {=} Q_{Z_2}, P_Y {=}  Q_{Y} \} $ and $ \gQ_2 {=} \{Q(Z_2|Y) | Q_{Z_1} {=} P_Z {=} Q_{Z_2}, P_X {=} Q_{X}\} $ are the set of all probabilistic encoders, where $ Q_{Z_1} $ and $ Q_{Z_2} $ are the marginal distributions of $ Z_1 {\sim} Q(Z_1|X) $ and $ Z_2 {\sim} Q(Z_2|Y) $, where $ X {\sim} P_{X}  $ and $ Y {\sim} P_{Y} $, respectively.  
	 
	Line (\ref{eqn:ae1}) uses the tower rule of expectation and Line (\ref{eqn:ae2}) holds by the conditional independence property of $ \gP_{X, X', Z} $. 
%	In line (\ref{eqn:ae3}), we take the expectation w.r.t. the models $ P(X|Z_1) $ and $ P(Y|Z_2) $, respectively.
	In line (\ref{eqn:ae4}), we take the expectation w.r.t. $ X' $ and $ Y' $, respectively, and use the total probability.
	Line (\ref{eqn:ae5}) follows the fact that $ \gP_{X, Z_1} {=} \gP(X {\sim} P_X, Z_1 {\sim} P_{Z_1}) $ and $ \gP_{Y, Z_2} {=} \gP(Y {\sim} P_Y, Z_2 {\sim} P_{Z_2}) $ since $ \gP(P_X, P_{G_1}), \gP_{X, X', Z_1} $ and $ \gP_{X, Y} $ depend on the choice of conditional distributions $ P_{G_1}(X'|Z_1) $, while $ P_{X, Z_1} $ does not, and likewise for distributions w.r.t. $ Y $ and $ G_2 $. 
	In line (\ref{eqn:ae6}), the generative model $ Q(Z_1|X) $ can be derived from two cases where $ Z_1 $ can be sampled from $ E_1(X) $ and $ E_2(G_2(E_1(X))) $ when $ Q_{Z_1} {=} Q_{Z_2} $ and $ P_Y {=} Q_{Y} $, and likewise for the generative model $ Q(Z_2|Y) $.
\end{proof}
%
%\section{Proof of Theorem \ref{theorem}}
%
%\begin{lemma}\label{lemma:dual_KR}
%	Given an $ L_{c_2} $-Lipschitz cost function $ c_2 $, a probabilistic cross-domain Lipschitz function $ f^* $, and two joint distributions $ P_{\gA}^f $ and $ P_{\gB}^g $ w.r.t. $ f $ and $ g $, respectively, then for any coupling $ P( X, Y^f; X^g, Y) \in \gP(P_{\gA}^f, P_{\gB}^g) $, we have
%	\begin{align*}
%		\left| \int_{\gX \times \gY} c_2 (Y, f^*(X)) d ( P_{\gA}^f {-} P_{\gB}^g ) \right| 
%		{\leq} \int_{(\gX \times \gY)^2} \left| c_2 (Y^f, f^*(X)) {-} c_2(Y, f^*(X^g)) \right|d P( X, Y^f; X^g, Y),
%	\end{align*}
%	where $ P_{\gA}^f {=} (X, Y^f)_{X \sim P_X} $ and $ P_{\gB}^g {=} (X^g, Y)_{Y {\sim} P_Y}  $, and $ Y^f {=} f(X) $ and $ X^g {=} g(Y) $.
%\end{lemma}
%\begin{proof}
%	Given joint distributions $ P_{\gA}^f {=} (X, f(X))_{X \sim P_X} $ and $ P_{\gB}^g {=} (g(Y), Y)_{Y {\sim} P_Y} $, and an $ L_{c_2} $-Lipschitz cost function $ c_2 $ on $ \gY \times \gY $, 
%	and based on the duality form of the Kantorovitch-Rubinstein theorem \cite{rachev1990duality, villani2008optimal}, we have
%	\begin{align*}
%	\sup \int_{\gX \times \gY} c_2 (Y, f^*(X)) d ( P_{\gA}^f - P_{\gB}^g ) 
%	= \inf \int_{(\gX \times \gY)^2} d_{f^*}(X, Y^f; X^g, Y) d P (X, Y^f; X^g, Y)
%	\end{align*}
%	where $ d_{f^*}(X, Y^f; X^g, Y) $ is a cost function of $ f^* $ w.r.t. $ (X, Y^f; X^g, Y) $, and the cost function $ c_2 $ satisfies the condition, \textit{i.e.}, $ c_2 (Y^f, f^*(X)) - c_2 (Y, f^*(X^g)) \leq d_{f^*} (X, Y^f; X^g, Y) $. Specifically, we choose its equality , then we have
%	\begin{align*}
%		& \left|\int_{\gX \times \gY} c_2 (Y, f^*(X)) d ( P_{\gA}^f - P_{\gB}^g ) \right|\\
%		\leq& \left| \int_{(\gX \times \gY)^2} c_2 (Y^f, f^*(X)) - c_2 (Y, f^*(X^g)) d P (X, Y^f; X^g, Y) \right|\\
%		\leq& \int_{(\gX \times \gY)^2} \left|  c_2 (Y^f, f^*(X)) - c_2 (Y, f^*(X^g)) \right| d P (X, Y^f; X^g, Y).
%	\end{align*}
%\end{proof}
%
%\begin{lemma}
%	Given an $ L_{c_1} $-Lipschitz cost function $ c_1 $, two joint distributions $ P_{\gA}^f $ and $ P_{\gB}^g $, and a $ \phi(\alpha) $-probabilistic cross-domain Lipschitz function $ f^* $, we assume the input space $ \gX $ is bounded such that $ \| f^*(X_1) - f^*(X_2) \| \leq M_1 $, then we have
%	\begin{align*}
%	\left| E_{\gA}^f (f^*) - E_{\gB}^g (f^*) \right| \leq \gW (P_{\gA}^f, P_{\gB}^g) + L_{c_1} M_1 \phi(\alpha).
%	\end{align*}
%\end{lemma}
%\begin{proof}
%	Based on the definition of $ E_{\gA}^f (f^*) $ and $ E_{\gB}^g (f^*) $, we discuss the absolute value of the difference between them as follows:
%	\begin{small}
%	\begin{align}
%	&\left| E_{\gA}^f (f^*) - E_{\gB}^g (f^*) \right| \nonumber \\
%	=& \left| \E_{(X, Y) \sim P_{\gA}^f(X, Y)} \left[ c_2 (Y, f^*(X)) \right] - \E_{(X, Y) \sim P_{\gB}^g(X, Y)} \left[ c_2 (Y, f^*(X)) \right] \right| \nonumber\\ 
%%	=& \left| \int_{\gX \times \gY} c_2 (Y, f^*(X)) \left( p_{\gA}^f(X, Y) - p_{\gB}^g(X, Y) \right) d X d Y \right| \\
%	=& \left| \int_{\gX \times \gY} c_2 (Y, f^*(X)) d \left( P_{\gA}^f - P_{\gB}^g \right) \right| \label{eqn. c1}\\
%	\leq& \int_{(\gX \times \gY)^2} \left| c_2 (Y^f, f^*(X)) - c_2(Y, f^*(X^g)) \right| d P^* (X, Y^f; X^g, Y) \label{eqn. c2} \\
%	=& \int_{{(\gX \times \gY)^2}} \left| c_2 (Y^f, f^*(X)) -  c_2 (Y^f, f^*(X^g)) {+} c_2 (Y^f, f^*(X^g)) - c_2(Y, f^*(X^g)) \right| d P^* (X, Y^f; X^g, Y) \nonumber\\
%	\leq& \int_{(\gX \times \gY)^2} \left| c_2 (Y^f, f^*(X)) {-} c_2 (Y^f, f^*(X^g)) \right| {+} \left| c_2 (Y^f, f^*(X^g)) {-} c_2(Y, f^*(X^g)) \right| d P^* (X, Y^f; X^g, Y) \nonumber\\
%	\leq& \int_{(\gX \times \gY)^2} \left[ L_{c_2} \left\| f^*(X) {-} f^*(X^g) \right\| {+}  c_2 (Y^f, Y) \right] d P^* (X, Y^f; X^g, Y) \label{eqn. c3}\\
%	\leq& \int_{(\gX \times \gY)^2} \left[ L_{1} \alpha c_1(X, X^g) {+} c_2 (Y^f, Y) \right] d P^* (X, Y^f; X^g, Y) {+} L_{1} M_1 \phi (\alpha)   \label{eqn. c4}\\
%	\leq& \int_{(\gX {\times} \gY)^2} \left[ c_1 (X^g, X) {+} c_2 (Y, Y^f) \right] d P^* (X, Y^f; X^g, Y) + L_{1} M_1 \phi(\alpha) \label{eqn. c5}\\
%	=& \gW (P_{\gA}^f, P_{\gB}^g) {+} L_{1} M_1 \phi(\alpha). \label{eqn. c6}
%	\end{align}
%	\end{small}
%    Line (\ref{eqn. c1}) follows by the definition of $ E_{\gA}^f (f^*) $ and $ E_{\gB}^g (f^*) $ and the definition of the expectation w.r.t. $ P_{\gA}^f $ and $ P_{\gB}^g $.
%    Line (\ref{eqn. c2}) holds by Lemma \ref{lemma:dual_KR} and we choose the optimal coupling $ P^* $, \textit{i.e.},
%    \begin{align*}
%	    P^* = \argmin\nolimits_{P \in \gP(P_{\gA}^f, P_{\gB}^g)} \E_{(X, Y'; X', Y) \sim P} [ c(X, Y'; X', Y) ].
%    \end{align*}
%	Line (\ref{eqn. c3}) holds by the $ L_{c_2} $-Lipschitz cost function $ c_2 $ w.r.t. the second argument, \textit{i.e.},
%	\begin{align*}
%	\left| c_2 (Y^f, f^*(X)) -  c_2 (Y^f, f^*(X^g)) \right| \leq L_{c_2} \left| f^*(X) - f^*(X^g) \right|,
%	\end{align*}
%	and the triangle inequality of the cost $ c_2 $, \textit{i.e.}, $ | c_2(Y^f, f^*(X^g)) - c_2(Y, f^*(X^g))| \leq c_2(Y^f, Y) $. 
%	Based on Definition \ref{def:probabilistic_Lipschitzness}, line (\ref{eqn. c4}) contains two cases: (1) $ f^* $ and $ \gP^* $ satisfies the  $ \phi $-probabilistic cross-domain Lipschitzness with probability $ 1 - \phi(\alpha) $; (2) the difference of $ f^* $ between any two instances is bounded by $ M_1 $, and we have the additional term $ L_{c_1} M_1 \phi (\alpha) $ that covers the regions where the $ \phi $-probabilistic cross-task Lipschitzness does not hold, \textit{i.e.}
%	\begin{align*}
%	& \int_{(\gX \times \gY)^2} L_{c_1} \left| f^*(X) - f^*(X^g) \right| d P^* (X, Y^f; X^g, Y) \\
%	\leq& \int_{(\gX \times \gY)^2} L_{c_1} \alpha c_2(X, X^g) d P^* (X, Y^f; X^g, Y) + L_{c_1} M_1 \phi (\alpha).
%	\end{align*}
%	Line (\ref{eqn. c5}) holds by the Lipschitz cost function $ c_1 $, and line (\ref{eqn. c6}) uses the definition of $ \gW (P_{\gA}^f, P_{\gB}^g) $.
%\end{proof}
%
%\begin{lemma}\label{Lemma:E_A_B}
%	Given Lipschitz cost function $ c_1 $ and $ c_2 $, and the input instances are bounded for $ f^* $ and $ g^* $, \textit{i.e.}, $ \|f^* (\bx_1) {-} f^* (\bx_2)\| \leq M_1 $ and $ \|g^* (\by_1) {-} g^* (\by_2)\| \leq M_2 $, if $   L_{c_1} \alpha {=} L_{c_2} \beta {=} 1 $, we have 
%	\begin{align*}
%	&E_{\gA}(f) \leq \gW_c (P_{\gA}^f, P_{\gB}^g) + L_{c_1} M_1 \phi (\alpha) + E_{\gA} (f^*) + E_{\gB}^g (f^*),\\
%	&E_{\gB}(g) \leq \gW_c (P_{\gA}^f, P_{\gB}^g) + L_{c_2} M_2 \phi (\beta)  + E_{\gB} (g^*) + E_{\gA}^f (g^*),
%	\end{align*}
%	with probability at least $ 1 - \delta $. 
%\end{lemma}
%\begin{proof}
%	Given $ E_{\gA}(f) = \E_{(X, Y) \sim P_{\gA}} \left[ c_2 (Y, f(X)) \right] $ and $ E_{\gB}(g) = \E_{(X, Y) \sim P_{\gB}} \left[ c_1 (X, g(Y)) \right] $, without loss of generality, we analyze the former as follows, and the latter is similar for the results.
%	\begin{align}
%	E_{\gA} (f)   
%	=& \E_{(X, Y) \sim P_{\gA}} \left[ c_2 (Y, f(X)) \right] \nonumber\\
%	=& \E_{(X, Y) \sim P_{\gA}} \left[ c_2 (Y, f^*(X)) + c_2 (f^*(X), f(X) ) \right] \label{l2eqn. 1}\\
%	=& \E_{(X, Y) \sim P_{\gA}} \left[ c_2 (f(X), f^*(X)) \right] + E_{\gA} (f^*)  \label{l2eqn. 2}\\
%	=& \E_{(X, Y) \sim P_{\gA}^f} \left[ c_2 (f(X), f^*(X) \right] + E_{\gA} (f^*) \label{l2eqn. 3} \\
%	=& E_{\gA}^f (f^*) + E_{\gA} (f^*)  \nonumber\\ 
%	=& E_{\gA}^f (f^*) - E_{\gB}^g (f^*) + E_{\gB}^g (f^*) + E_{\gA} (f^*)  \nonumber\\ 
%	\leq& \left| E_{\gA}^f (f^*) - E_{\gB}^g (f^*) \right| + E_{\gB}^g (f^*) + E_{\gA} (f^*) \label{l2eqn. 4} \\
%	\leq& \gW_c (P_{\gA}^f, P_{\gB}^g) + L_{1} M_1 \phi(\alpha) + E_{\gB}^g (f^*) + E_{\gA} (f^*).
%	\end{align}
%	Line (\ref{l2eqn. 1}) holds by an assumption that the loss function $ c_1 $ satisfies triangle inequality. 
%	Line (\ref{l2eqn. 2}) holds by a symmetric loss function $ c_1 $ and the definition of $ E_{\gA} (f^*) $, \textit{i.e.}, $ E_{\gA} (f^*) = \E_{(X, Y) \sim P_{\gA}} [c_2 (Y, f^*(X)] $.
%	Line (\ref{l2eqn. 3}) uses a fact that 
%	\begin{align*}
%	  \E_{(X, Y) \sim P_{\gA}} \left[ c_2 (f(X), f^*(X)) \right] 
%	= \E_{(X, f(X)) \sim P_{\gA}^f} \left[ c_2 (f(X), f^*(X)) \right] 
%	= E_{\gA}^f (f^*).
%	\end{align*}
%\end{proof}
%In order to prove Theorem \ref{theorem}, we introduce an important theorem that shows the concentration inequality for Wasserstein distance of the empirical measure and its true measure.
%\begin{thm} \emph{\textbf{(Empirical Concentration \cite{bolley-PTRF2007-quantitative}, Theorem 1.1)}}
%	\label{theorem: concentration_W}
%	Let $ \mu $ be a probability measure on $ \Omega $ 
%%	so that for some $ \rvw \in \Omega $, we have 
%%	\[\int e^{\tau d(\bw, \bw')^2} d \mu(\rvw) < +\infty,  \tau > 0 \]
%%	for any $ \rvw' \in \Omega $, 
%	and $ \hat{\mu} = \frac{1}{N} \sum_{i=1}^{N} \delta_{\rvw_i} $ be the associated empirical measure defined on a sample of independent variables $ \{\rvw_i\}_{i=1}^N $ drawn from $ \mu $. Then, for any $ d' > dim(\Omega) $ and $ C' < C $, there exists some constant $ N_0 $ depending on $ d' $ and some square exponential monments of $ \mu $ such that for any $ \epsilon > 0 $ and $ N \ge N_0 \max \{\epsilon^{-(d' + 2)}, 1\} $,
%	\begin{align*}
%	P\left[ \gW (\mu, \widehat{\mu}) > \epsilon \right] \leq e^{-\frac{C'}{2} N \epsilon^2},
%	\end{align*}
%	where $ C' $ can be calculated explicitly, and $ C $ is such that $ \mu $ verifies for any measure $ \nu $ the Talagrand (transportation) inequality $ T_1(C):  \gW(\mu, \nu) {\leq} {(\frac{2}{C} H(\nu|\mu))^\frac{1}{2}} $ with the relative entropy $ H $, and $ T_1(C) $ holds when for some $ \tau > 0 $ and $ \int e^{\tau d(\bw, \bw')^2} d \mu(\rvw) {<} {+}\infty, \forall\; \rvw' {\in} \Omega $.
%\end{thm}
%This theorem allows us to propose generalization bounds based on the Wasserstein distance.
%Now we can use this theorem and the previous Lemma to prove the following theorem.
%\begin{thm}\label{theorem}
%	Let $ P^* {=} \argmin_{P \in \gP(P_{\gA}^f, P_{\gB}^g)} \E_{(X, Y^f; X^g, Y) \sim P} [ c(X, Y^f; X^g, Y) ] $ with Lipschitz cost functions $ c_1 $ and $ c_2 $, and let functions $ f^* {\in} \gF $ and $ g^* {\in} \gG $ be probabilistic cross-domain Lipschitzness w.r.t. $ P^* $ that minimizes the joint error $ E(f^*, g^*) $, 
%	given $ M $ instances and $ N $ instances drawn form $ P_X $ and $ P_Y $, respectively, with $ L_{c_1} \alpha {=} L_{c_2} \beta {=} 1$, we have with probability at least $ 1 {-} \delta $:
%	\begin{align*}
%	E(f, g) \leq 2W_1 (\widehat{P}_{\gA}^f, \widehat{P}_{\gB}^g) + \sqrt{\frac{2}{C'} \log \left( \frac{2}{\delta} \right)} \left( \frac{2}{\sqrt{M}} + \frac{2}{\sqrt{N}} \right) + E(f^*, g^*) + \tilde{\phi} (\alpha, \beta), 
%	\end{align*}
%	where $ E(f^*, g^*) {=} E_{\gA} (f^*) {+} E_{\gB}^g (f^*) {+} E_{\gB} (g^*) {+} E_{\gA}^f (g^*) $, and $ \tilde{\phi} (\alpha, \beta) {=} L_{c_1} M_1 \phi (\alpha) {+} L_{c_2} M_2 \phi (\beta) $, where $ \| f^*(X_1) - f^*(X_2) \| \leq M_1, \forall X_1, X_2 \in \gX $ and $ \| g^*(Y_1) {-} g^*(Y_2) \| {\leq} M_2, \forall Y_1, Y_2 {\in} \gY $. Here, $ C' $ is some constant satisfying Theorem \ref{theorem: concentration_W}.
%\end{thm}
%\begin{proof}
%%	Let $ E(f^*, g^*) {=} E_{\gA} (f^*) {+} E_{\gB}^g (f^*) {+} E_{\gB} (g^*) {+} E_{\gA}^f (g^*) $, and $ \tilde{\phi} (\alpha, \beta) {=} L_{c_1} M_1 \phi (\alpha) {+} L_{c_2} M_2 \phi (\beta) $. 
%	Based on the definition of $ E(f, g) $, we have
%	\begin{align}
%	E(f, g) =& \E_{(X, Y) \sim P_{\gA}} \left[ c_2 (Y, f(X)) \right] + 
%	\E_{(X, Y) \sim P_{\gB}} \left[ c_1 (X, g(Y)) \right] \nonumber\\
%	\leq& 2 \gW (P_{\gA}^f, P_{\gB}^g) + E(f^*, g^*) + \tilde{\phi} (\alpha, \beta) \label{thm1:1}\\
%	\leq& 2 \gW (\widehat{P}_{\gA}^f, \widehat{P}_{\gB}^g) + \gW (\widehat{P}_{\gA}^f, P_{\gA}^f) \small{+} \gW (\widehat{P}_{\gB}^g, P_{\gB}^g) {+} E(f^*, g^*) {+} \tilde{\phi} (\alpha, \beta) \label{thm1:2}\\
%	\leq& 2 \gW (\widehat{P}_{\gA}^f, \widehat{P}_{\gB}^g) + \sqrt{\frac{2}{t'} \log \left( \frac{2}{\delta} \right)} \left( \frac{2}{\sqrt{M}} + \frac{2}{\sqrt{N}} \right) + E(f^*, g^*) + \tilde{\phi} (\alpha, \beta) \label{thm1:3}.
%	\end{align}
%	Line (\ref{thm1:1}) holds by the conclusion in Lemma \ref{Lemma:E_A_B}, and
%	line (\ref{thm1:2}) uses the triangle inequality for $ 1 $-Wasserstein distance.
%	In line (\ref{thm1:3}), we apply the union bound of $ \gW (\widehat{P}_{\gA}^f, P_{\gA}^f) $ and $ \gW (\widehat{P}_{\gB}^g, P_{\gB}^g) $ (with probability $ \frac{\delta}{2} $ for each) in Theorem \ref{theorem: concentration_W}.
%\end{proof}

\newpage
\section{Optimization Details}
In this section, we discuss some details of optimization for distribution divergence.
In the training, we use original GAN to measure the divergence $ d(P_X, Q_{X}) $, $ d(P_Y, Q_{Y}) $ and $ d(P_Z, Q_{Z}) $, respectively.

For $ d(P_X, Q_{X}) $, we optimize the following minimax problem:
\begin{align}
&\min_{F} \max_{D_x} \left[ \hat{\E}_{\bx \sim P_X} [\log D_x (\bx)] + \hat{\E}_{\tilde{\bx} \sim Q_X} [\log(1-D_x(\tilde{\bx}))] \right] \\
=&\min_{F} \max_{D_x}\left[ \hat{\E}_{\bx \sim P_X} [\log D_x (\bx)] + \lambda \hat{\E}_{{\bx} \sim P_X} [\log(1-D_x(G_1(E_2(G_2(E_1(\bx)))))))] + (1{-}\lambda) \hat{\E}_{{\by} \sim P_Y} (1{-}D_x(G_1(E_2(\by)))) \right],\nonumber
\end{align}
where $ D_x $ is a discriminator \wrt $ X $, and $ \lambda \in (0, 1) $.


For $ d(P_Y, Q_{Y}) $, we optimize the following minimax problem:
\begin{align}
&\min_{F} \max_{D_y} \left[ \hat{\E}_{\by \sim P_Y} [\log D_y (\by)] + \hat{\E}_{\tilde{\by} \sim Q_Y} [\log(1-D_y(\tilde{\by}))] \right] \\
=&\min_{F} \max_{D_y}\left[ \hat{\E}_{\by \sim P_Y} [\log D_y (\by)] + \lambda \hat{\E}_{{\by} \sim P_Y} [\log(1-D_y(G_2(E_1(G_1(E_2(\by)))))))] + (1{-}\lambda) \hat{\E}_{{\bx} \sim P_X} (1{-}D_y(G_2(E_1(\bx)))) \right],\nonumber
\end{align}
where $D_y$ is a discriminator \wrt $Y$, and $ \lambda \in (0, 1) $.


For $ d(P_Z, Q_{Z}) $, it contains $ d(P_Z, Q_{Z_1}) $ and $ d(P_Z, Q_{Z_2}) $ simultaneously, we optimize the following minimax problem:
\begin{align*}
	d(P_Z, Q_{Z_1}){=}\min_{E_1} \max_{D_z} \left[ \hat{\E}_{\bz \sim P_Z} [\log D_z (\bz)] + \hat{\E}_{{\bx} \sim P_X} [\log(1-D_z(E_1(\bx)))] \right],
\end{align*} 
where $D_z$ is a discriminator \wrt $Z$, and $ \rvz  $ is drawn from the prior distribution $ P_{Z} $.
Similarly, the another term $ d(P_Z, Q_{Z_2}) $ can be written as
\begin{align*}
d(P_Z, Q_{Z_2}){=}\min_{E_2} \max_{D_z} \left[ \hat{\E}_{\bz \sim P_Z} [\log D_z (\bz)] + \hat{\E}_{{\by} \sim P_Y} [\log(1-D_z(E_2(\by)))] \right].
\end{align*}
%Let $ {\gL_{z}}(E_1{,} E_2{,} G_1{,} G_1{,} D_{z}){=}{\gL_{z_1}}(E_1{,} E_2{,} G_2{,} D_{z}){+}{\gL_{z_2}}(E_1{,} E_2{,} G_1{,} D_{z}) $ be the final loss. %minimizing $ {\gL}_{z} $ is consistent with the shared-latent space assumption~\cite{liu2017unsupervised} that images of two different domains have the same latent representation distribution.
%Here, minimizing $ {\gL}_{z} $ is similar to~\cite{liu2017unsupervised} which uses VAE-like objective with the similar cycle-consistency constraint.
%Moreover, ~\cite{liu2017unsupervised} also optimize $ \gD_Z(P_Z, Q_{Z_1}) $ by VAE-like objective using the similar cycle constraint.

%\end{appendix}
